# Supplementary material for: On Optimizing the Trade-off between Privacy and Utility in Data Provenance
Source: arXiv:2103.00288 source file (2021-02-27)
Supplement: Supplementary file 1 [file appendix.tex]

\begin{proposition} \label{prop:concretization-set-size}
Given an abstraction tree $T$ that compatible with a \ex\ $Ex$ and an abstraction function $A_T$, it holds that:
\begin{enumerate}
    \item $|C(A_T(Ex))|=\displaystyle\prod_{v \in Var(Ex)}~|~L_T(A_T(v))|$
    \item $1 \leq |C(A_T(Ex))| \leq |L(T)|^n$ (bounds are tight), where $n=|\{v \in Var(Ex)~|~v \neq A_T(v)\}|$.
    % \item There exist abstraction functions $A_T', A_T''$ such that\\
    % $|C(A_T'(Ex))|=1$ and $|C(A_T''(Ex))|=|L(T)|^n$.
\end{enumerate}
\end{proposition}
